# Supplementary material for: CoRCi: Cross-Reconstruction of Coherent Interests Modeling in Cross-Domain Sequential Recommendation
Source: arXiv:2608.09580 source file (2026-08-10)
Supplement: Supplementary file 1 [file ch7_appendix.tex]

%
%----------------------------------------------------------
\section{Hyperparameters Sensitivity analysis}
%----------------------------------------------------------
%
%----------------------------------------------------------
\subsection{Sequence Length $L$} \label{app: len}
%----------------------------------------------------------
%
%----------------------------------------------------------
\subsection{Embedding Size $d$} \label{app: emb}
%----------------------------------------------------------
%

%
%----------------------------------------------------------
\section{Running Time} \label{app: time}
%----------------------------------------------------------
%
